# Supplementary material for: Image Synthesis with a Single (Robust) Classifier
Source: arXiv:1906.09453 source file (2019-08-08)
Supplement: Supplementary file 1 [file appendix.tex]

\section{Experimental Setup}

\subsection{Inpainting}
\label{app:inpaint_setup}
